# Supplementary material for: Fair Leader Election for Rational Agents in Asynchronous Rings and Networks
Source: arXiv:1805.04778 source file (2018-05-15)
Supplement: Supplementary file 1 [file appendix-uni-vs-bi.tex]

In order to elect a leader in a bidirectional ring, we embed a
unidirectional ring in it. The other direction is not trivial. The
following building block gives a reason to believe that a
unidirectional ring is as strong as a bidirectional ring. I.e., if
there is an \kresilient fair coin toss protocol for a bidirectional
ring then there is an \kresilient fair coin toss protocol for a
unidirectional ring. Note that the other direction is true because
one can embed a unidirectional ring in a bidirectional ring.

We explain how to simulate a bidirectional ring on a unidirectional
ring. At initialization, each processor $b$ sends a huge secret
random string $S_b$ to its successor $a$. Later $a$ will use it as a
one-time pad to send perfectly encrypted messages to $b$. During the
simulation, if a processor $a$ wants to send a message $M \in
\{0,1\}^L$ to its predecessor $b$, then it takes the next unused
prefix of the random string $S_b$, $x \in \{0, 1\}^L$, and sends $x
\oplus M$ along the unidirectional ring. Upon receiving the message,
$b$ deciphers its content and send $M$ to $a$, so $a$ can validate
the message reached its destination untempered.

Maybe this idea can be expanded to create a reduction. The question
is not trivial because while the content of messages cannot be read
or changed, still two adjacent adversaries can abuse this mechanism
to send information along the ring in the opposite direction. A
