# Supplementary material for: Fair Leader Election for Rational Agents in Asynchronous Rings and Networks
Source: arXiv:1805.04778 source file (2018-05-15)
Supplement: Supplementary file 2 [file appendix-verbose-model.tex]

For completeness, we include a detailed definition of the model. The
proofs do not use this definition directly, so it may be skipped.

Some of the processors wake-up spontaneously and execute their
\emph{Init()} procedure. In the \emph{Init()} procedure, a processor
may send messages. The rest of the processors wake-up upon receiving
the first message, and execute their \emph{Init()} procedure. After
a processor woke up or received its first incoming message, it
cannot wake up spontaneously.

Additionally, each processor receives a private input, which depends
on the problem.

A \textbf{message schedule} is a vector of $2|E|$ scheduling functions - a function for each direction of each FIFO link. Every scheduling function is of the form $f_{p, q}:\mathbb{R}_+\times \mathbb{N} \to \mathbb{R}$, where $f_{p, q}(t, i)$ denotes the arrival time of the $i^{th}$ message (if it exists) that $p$ sent to $q$ at time $t$. Every such function is monotonic in both entries and upholds $\forall t\in \mathbb{R}_+: f_{p,q}(t, 1) > t$, $\forall t>s>0, i\in \mathbb{N}:f_{p,q}(t, 1) > f_{p,q}(s, i) $. Additionally, in order to resolve ambiguity due to simultaneous delivery of messages, we require that the images $\{Image(f_{p,q})\}_{p,q\in V}$ are disjoint.\\

An \textbf{oblivious schedule} is a pair - a message schedule and a
vector of wake up times i.e., a spontaneous wake up time for each
processor.

In order to define an execution of a protocol, first we define a
single event. There are four types of \textbf{event}s - a type for
wake up, a type for sending a message, a type for receiving a
message and a type for termination. The first type is denoted by
$wakeup(A)$, it means that processor $A$ wakes up spontaneously. The
second type is denoted by $send(A,M,B)$, it means that processor $A$
sends the message $M$ to processor $B$. The third type is denoted by
$recv(A,M,B)$, it means that processor $B$ receives the message $M$
from processor $A$. The last type is denoted by $terminate(A,
out_0)$, it means that processor $A$ terminates with $output=out_0$.

Given a protocol $P$, a set of $id$s, a private inputs vector, an
\textbf{execution} of the protocol $P$ is a list of events (possibly
infinite) that conforms to the protocol's definition. One can think
of it as the full history of the protocol run. If the list is
finite, then every processor must have terminated or be idle. While
an idle processor, is a processor that all its incoming links are
empty, i.e., it has finished processing all its incoming messages.

Note that an execution is determined uniquely given: the $id$s, the
inputs, the protocol, a schedule, and the results of the local
randomizations.

Next, we generalize the definition above for protocols with
non-trivial private inputs.

Note that adversaries can always deviate from any protocol simply by behaving as if they got another input, that is they can select their input. Honest processors cannot distinguish such a behavior from an honest behavior, so no algorithm can provide any resilience guarantee against such cheating strategy. Therefore, resilience of a protocol with non-trivial inputs means that every coalition of size $\leq k$, cannot increase significantly the utility of all its members compared to the best utilities it could achieve simply by selecting the coalition's inputs.\\

Given an inputs vector $v$ and a coalition $C$, denote by $Adv_C(v)$ the set of all input vectors that differ from $v$ only in inputs of $C$.\\
Denote with $g^i(s, v)$ the payoff of processor $i$ (the expectancy
of its utility), when running the protocol $s$ while using the input
$v$.

\begin{definition}{(\kResilience - extended definition)}
    A symmetric protocol with inputs $P_{sym}$  is \kresilient if for every set of $id$s, for every vector of rational utility functions, for every oblivious schedule, for every inputs vector $v$, for every $C\subseteq \{1,... n\}$ such that $|C|\leq k$ and for all $s_C\in \prod_{j\in C}S^j$ there exists an agent $i\in C$ such that $max_{v'\in Adv_C(v)}g^i(s^*, v') + \epsilon \geq g^i(<s_C, s^*_{[n]\backslash C}>, v)$
\end{definition}

Two notes about the resilience definition.
\begin{itemize}
    \item We require that a deviating coalition cannot improve significantly the utility of every member in the coalition. Since we require this for every vector of rational utility functions, it is equivalent to a stronger requirement - a deviating coalition cannot to improve significantly the utility of any single member in the coalition.
    \item We require resilience to hold for \textit{every oblivious schedule}. Adversarial processors might use this requirement to communicate information using this side-channel although they do not know the ``time''. For example, consider the following diamond topology: $V=\{a, b, c, d, e\}, E=\{\{a,b\},\{a,c\},\{b,d\},\{c,d\}, \{d,e\}\}$, and the adversarial coalition $C=\{a,d\}$. Assume processor $e$ sends two messages to $d$, $m1, m2$, and assume processors $b,c$ just forward every message from $d$ to $a$. Set the schedule to create a considerable time gap between the arrival of $m1$ and $m2$. Also, set the schedule to forward messages on the rest of the links really quick. More, assume $d$ is expected to send the messages $m3, m4$ to $b$ and $c$ accordingly. Then $d$ can choose between the following two strategies:
    \begin{enumerate}
        \item Upon $recv(e, m1, d)$: $send(d, m3, b)$, and upon $recv(e, m2, d)$: $send(d, m4, c)$.
        \item Upon $recv(e, m1, d)$: $send(d, m4, c)$, and upon $recv(e, m2, d)$: $send(d, m3, b)$.
    \end{enumerate}
    Then, processor $a$ can calculate the chosen strategy by checking whether it received $m3$ before $m4$ or $m4$ before $m3$. Which means that processor $d$ communicated to $a$ another bit.
\end{itemize}

Note that the $n$ factor in Lemma \ref{Model:UnbiasResilienceEquiv}
is asymptotically tight. It is impossible to increase the
probability for \textit{every} outcome by $\epsilon$, but it might
be possible to increase the probability of all the outcomes but a
specific outcome by $\epsilon$ and decrease the probability of a
specific outcome by $n \epsilon$. Let $P$ be an \kunbiased FLE
protocol and let $D$ be a deviation from $P$ of size $k$. Consider
the following rational utility $u_p(j) = \mathbbm{1}[j \ne 1]$.
Assume we have for every $j\ne 1:
Pr_D(outcome=j)=\frac{1}{n}+\epsilon$ and $Pr_D(outcome=1) =
\frac{1}{n}-n \epsilon$. Then we have $E_D[u_p] = (n-1)(\frac{1}{n}
+ \epsilon) = E_P[u_p] + (n-1)\epsilon$.
